# Supplementary material for: Differentially Private Federated Knowledge Graphs Embedding
Source: arXiv:2105.07615 source file (2021-08-16)
Supplement: Supplementary file 1 [file Appendix.tex]

\clearpage
\appendix

%\section{Algorithm Explanation}
%\label{Appendix-Algorithm}
%In order to better understand the training procedure of the \ph{PPAT network}, we explain handshake mechanism between client and host KGs in Algorithm~\ref{DE_algo}.

\section{Baseline Results}\label{Appendix-Baseline}

We present the baseline accuracies of triple classification of the 11 knowledge graphs using TransE in Fig.~\ref{fig:baseline-transe}.
We can see that after adequate rounds of iterative training, the performances are difficult to be further improved though fluctuations and uncertainty exist.
The performances of baseline are unstable: accuracies of \emph{Yago} and \emph{Dbpedia} are even reduced.
Fig.~\ref{fig:fkge-baseline-more} shows the baseline performance of FKGE using different knowledge graph embedding models as base models. 
To verify the effectiveness of the proposed FKGE over unified structure of the knowledge graphs, we integrate 11 knowledge graphs into one united knowledge graph by merging aligned entities, and then test the performance of TransE on each KG independently.
The accuracy of triple classification of a unified knowledge graph is shown in Fig.~\ref{fig:unified}.
As shown in the Fig. ~\ref{fig:unified}, compared with the FKGE based on TransE in Fig. ~\ref{fig:fkge-transe}, the accuracy of triple classification in the unified knowledge embedding space has generally decreased by 8.78\% - 21.43\%.
Moreover, compared with the independent knowledge graph embedding in Fig.~\ref{fig:baseline-transe}, the unified knowledge graph embedding even has generally decreased by 6.82\% - 17.63\%.
The above comparative experiments show that, despite the aligned entities, integrating the embeddings of multiple knowledge graphs into one unified vector space does not help to obtain effective representation of the knowledge graphs for the triple classification.
%The reason of above results may be that different knowledge graphs are built for different domains.
%Intuitively, the shared knowledge may seem enhance each other, but according to our experiment, the distinct parts may introduce distractions for each other due to the heterogeneity of various knowledge graphs.

%Similar baseline accuracies of training through different KGE models (same as Figure~\ref{fig:fkge-trans-more}) and unified KGs together are shown in Figures~\ref{fig:fkge-baseline-more} and ~\ref{fig:unified}, respectively.

\begin{figure*}[h]
\setlength{\abovecaptionskip}{-0.15cm} %缩小caption和图像之间的距离
\centering
\subfigure[50 dimension.]{\label{sec:50-fkge}
\begin{minipage}[t]{0.32\linewidth}
\centering\vspace{-0.05in}
\includegraphics[width=6cm]{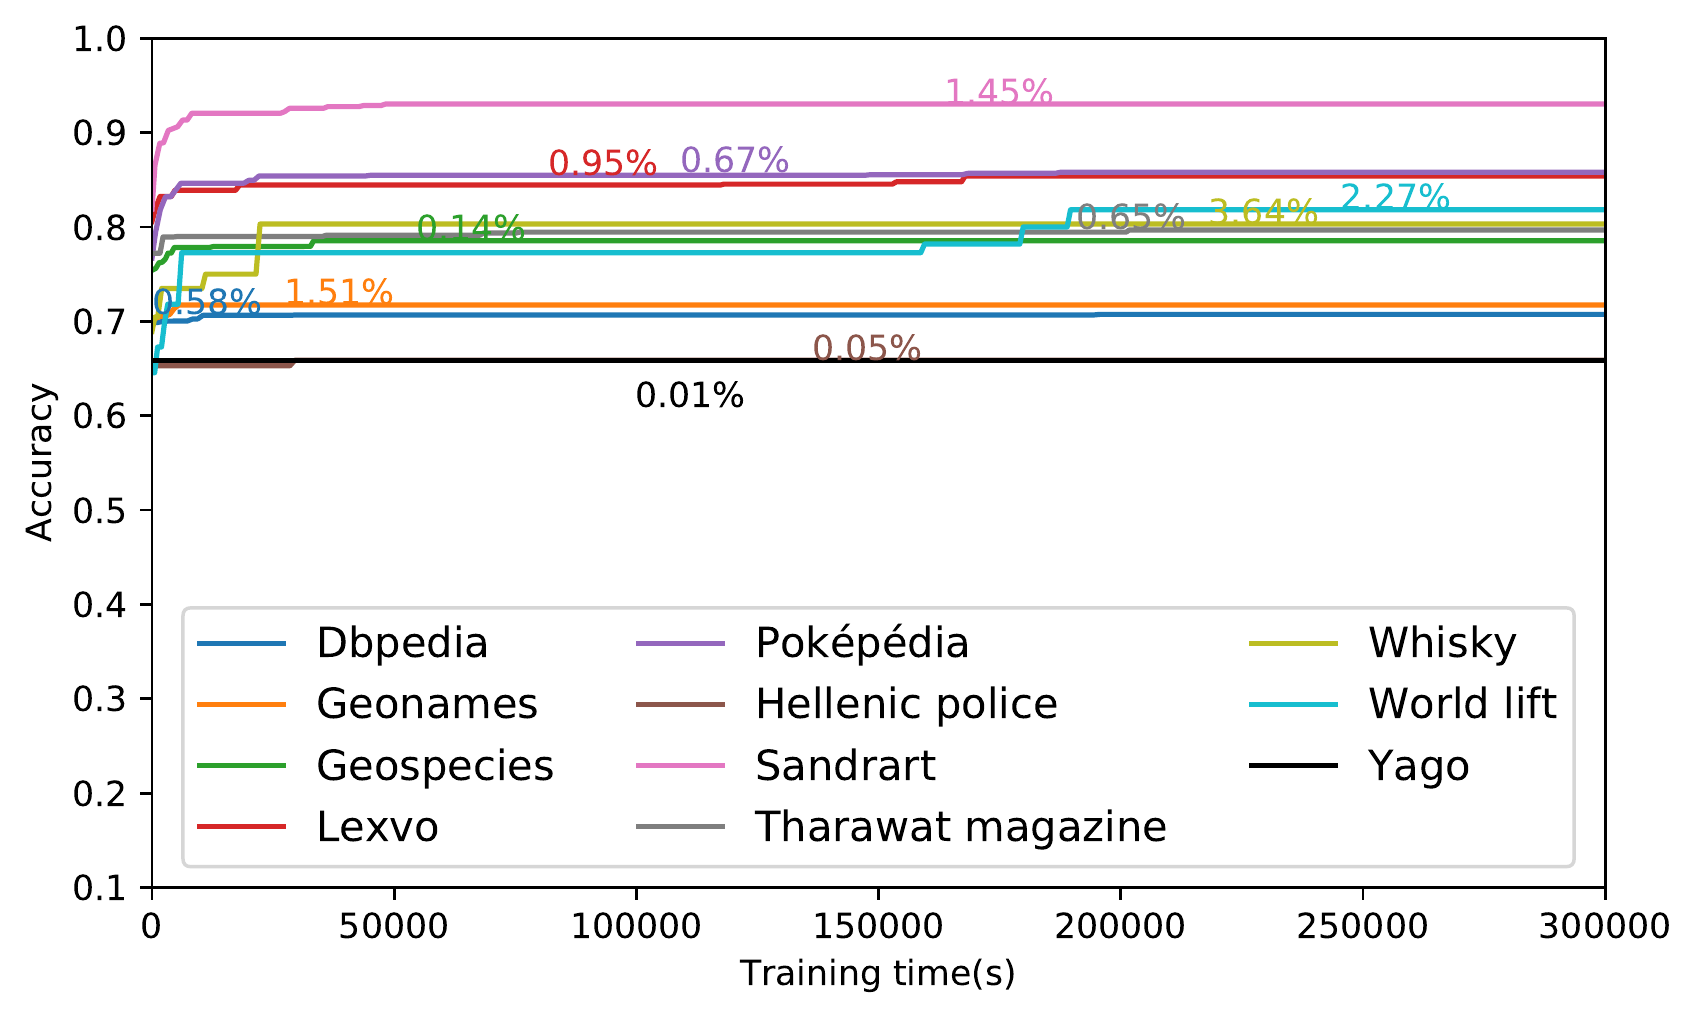}
\end{minipage}
}
\subfigure[200 dimension.]{\label{sec:200-fkge}
\begin{minipage}[t]{0.32\linewidth}
\centering\vspace{-0.05in}
\includegraphics[width=6cm]{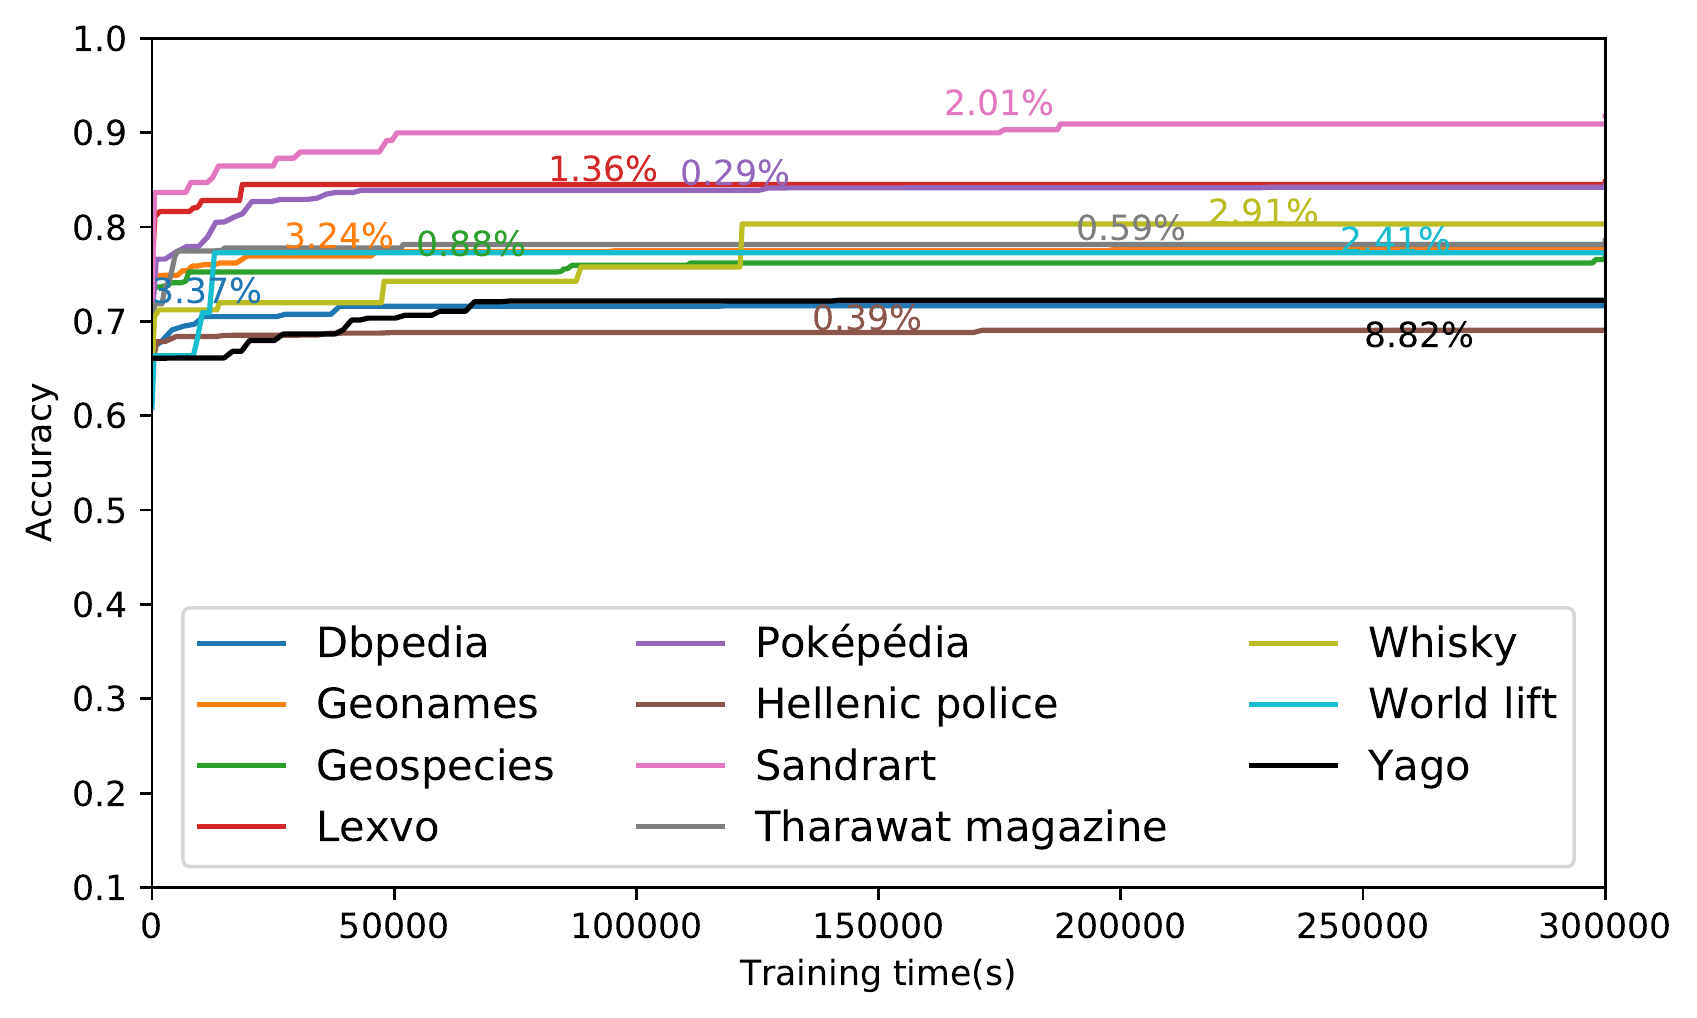}
\end{minipage}
}
\subfigure[300 dimension.]{\label{sec:300-fkge}
\begin{minipage}[t]{0.32\linewidth}
\centering\vspace{-0.05in}
\includegraphics[width=6cm]{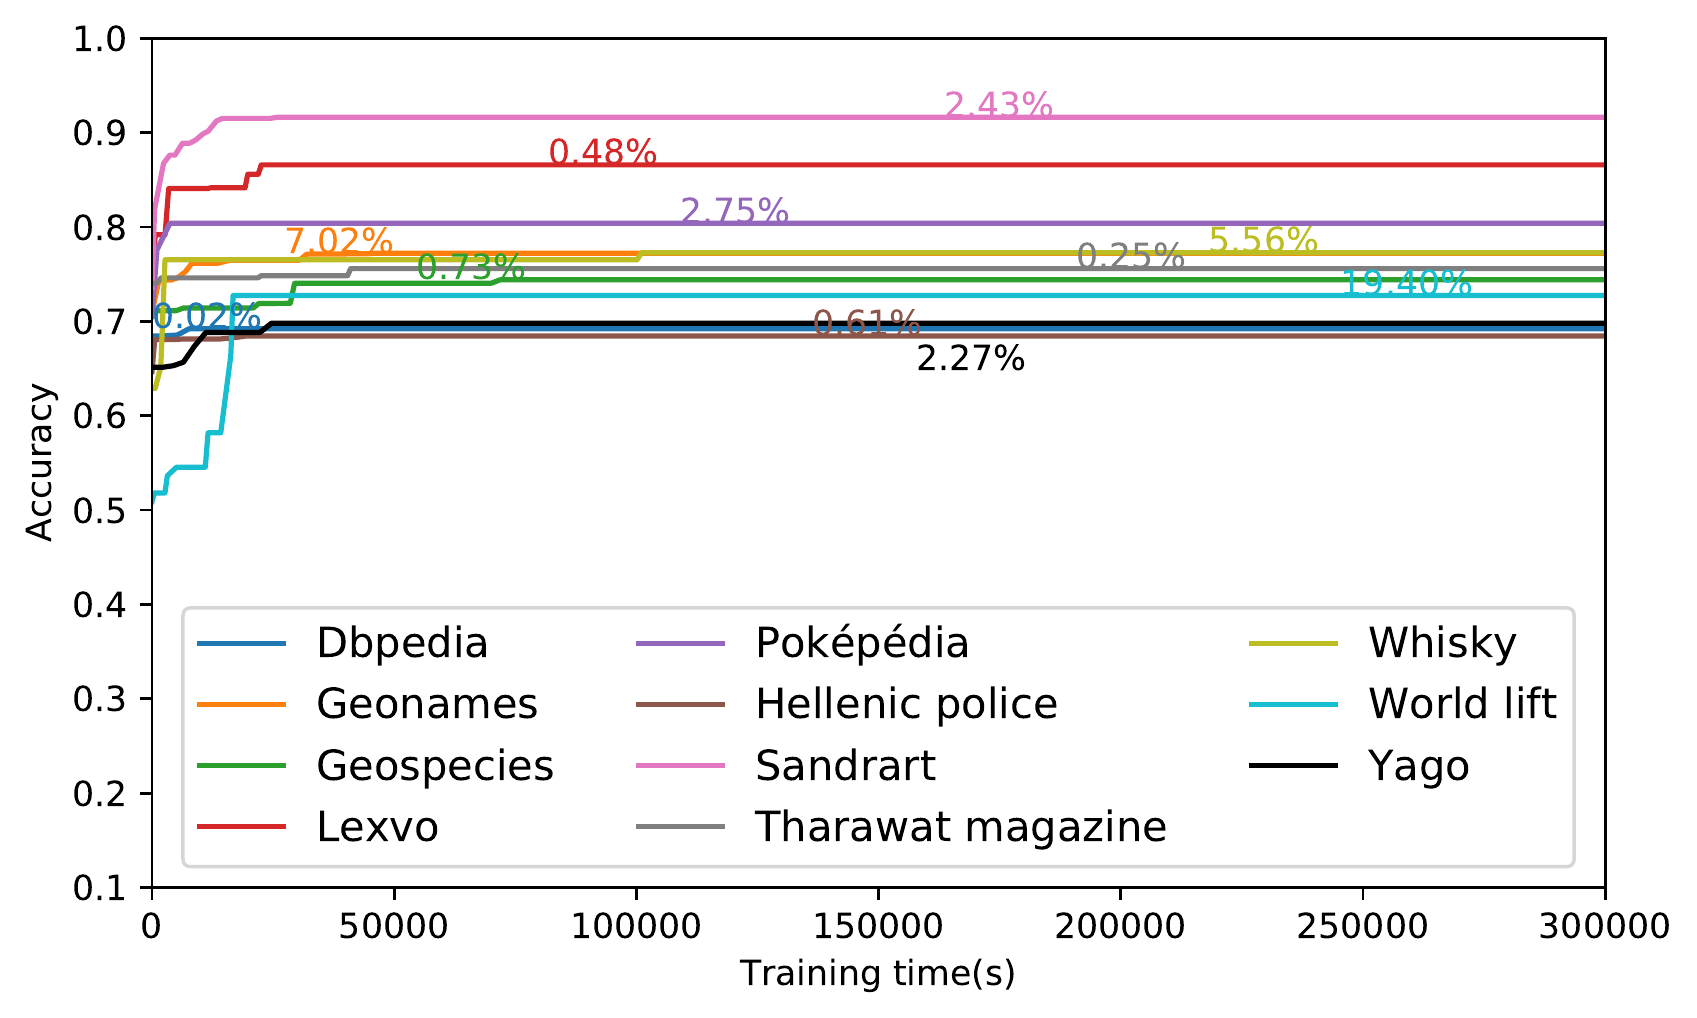}
\end{minipage}
}
\caption{Performance of FKGE using transE on triple classification with different dimensions of embedding vectors.}\label{fig:dimensions-fkge_old}
\end{figure*}

\begin{table*}[t]
	%\scriptsize
	\resizebox{1 \textwidth}{!}{
				\begin{tabular}{@{}c|c|cccc|cccc|cccc|cccc@{}}
			\toprule
			\multicolumn{2}{c|}{Sampling} & \multicolumn{4}{|c|}{\#20\%} & 	\multicolumn{4}{|c|}{\#40\%} & \multicolumn{4}{|c|}{\#60\%} & \multicolumn{4}{|c}{\#80\%}\\ \midrule
			\multicolumn{2}{c|}{Metric} & Mean Rank & Hit@10 & Hit@3 & Hit@1 & Mean Rank & Hit@10 & Hit@3 & Hit@1 & Mean Rank & Hit@10 & Hit@3 & Hit@1 & Mean Rank & Hit@10 & Hit@3 & Hit@1 \\ \midrule
		    %\multicolumn{2}{c|}{Dbpedia} & 6591.37 & 23.29 & 12.88 & 5.12 & 6454.12 & 23.81 & 13.12 & 5.34 & 6399.18 & 24.17 & 13.47 & 5.65 & 5981.02 & 24.26 & 13.63 & 5.81 & 6233.17 & 24.59 & 14.02 & 6.21 & 5833.17 & 25.07 & 14.41 & 6.37 \\ 
		    \multicolumn{2}{c|}{Geonames} & 
		    63,080.34 & 8.93 & 3.86 & 1.93 & 
		    62,421.95 & 9.17 & 4.47 & 1.99 & 
		    61,276.67 & 9.35 & 4.49 & 2.04 & 
		    59,786.04 & 9.65 & 4.57 & 2.04  \\
		    \multicolumn{2}{c|}{Yago} & 
		    30,638.51 & 2.05 & 0.76 & 0.25 &
		    28,838.64 & 2.235 & 0.79 & 0.26 & 
		    26,563.40 & 2.35 & 0.81 & 0.26 & 
		    26,421.51 & 2.55 & 0.82 & 0.27 \\
		    \multicolumn{2}{c|}{Geospecies} &
		    415.47 & 59.31 & 45.97 & 34.81 & 
		    409.06 & 59.70 & 45.99 & 35.08 & 
		    400.73 & 60.17 & 46.38 & 35.12 & 
		    397.69 & 60.28 & 46.72 & 35.30 \\
		    \multicolumn{2}{c|}{Poképédia} & 
		    7,463.42 & 38.37 & 30.01 & 20.01 & 
		    7,450.85 & 43.25 & 30.50 & 21.61 & 
		    7,445.54 & 44.09 & 33.08 & 23.39 & 
		    7,434.55 & 45.49 & 33.43 & 24.19 \\
		    \multicolumn{2}{c|}{Sandrart} & 
		    56.23 & 87.61 & 83.38 & 67.96 & 
		    52.39 & 88.38 & 83.43 & 69.51 & 
		    51.71 & 88.65 & 84.34 & 70.38 & 
		    47.39 & 88.98 & 84.37 & 72.10 \\
		    \multicolumn{2}{c|}{Hellenic Police} & 
		    1,886.24 & 32.29 & 22.06 & 19.03 & 
		    1,853.55 & 32.47 & 22.41 & 19.08 & 
		    1,823.84 & 32.63 & 22.78 & 19.11 & 
		    1,751.37 & 32.98 & 22.86 & 19.27 \\
		    \multicolumn{2}{c|}{Lexvo} &
		    43.64 & 86.01 & 76.59 & 58.43 & 
		    44.96 & 86.14 & 76.86 & 59.68 & 
		    43.43 & 86.70 & 77.11 & 60.47 & 
		    41.57 & 86.77 & 77.62 & 61.30 \\
		    \multicolumn{2}{c|}{Tharawat magazine} & 
		    232.63 & 12.50 & 4.58 & 1.76 & 
		    232.62 & 12.92 & 4.81 & 1.96 & 
		    228.65 & 13.13 & 5.09 & 1.99 & 
		    226.67 & 13.19 & 5.15 & 2.10 \\
		    \multicolumn{2}{c|}{Whisky} & 
		    49.47 & 29.39 & 15.98 & 9.91 & 
		    49.85 & 31.14 & 16.24 & 10.15 & 
		    44.47 & 31.85 & 17.06 & 10.25 & 
		    43.12 & 33.35 & 17.64 & 10.58 \\
		    \multicolumn{2}{c|}{World lift} &
		    22.98 & 46.80 & 25.47 & 7.85 & 
		    22.82 & 49.71 & 25.60 & 7.99 & 
		    22.74 & 50.06 & 28.62 & 8.02 & 
		    22.11 & 50.15 & 28.87 & 10.30 \\
		    \toprule
		\end{tabular}
	}\caption{Evaluation results on link prediction tasks in Filter with different sampling ratio(\%) of aligned entities.}\label{tab:link-scale-filter_old}
\vspace{-5mm}
\end{table*}

\begin{table*}[t]
	\resizebox{1 \textwidth}{!}{
		\begin{tabular}{@{}c|cccccccccccc@{}}
   		    \toprule
			\multicolumn{2}{c|}{KGs} & \multicolumn{1}{c}{Dbpedia}  & 
			\multicolumn{1}{c}{Geonames} & 
			\multicolumn{1}{c}{Yago} & 
			\multicolumn{1}{c}{Geospecies}& 
			\multicolumn{1}{c}{Poképédia} &
		    \multicolumn{1}{c}{Sandrart} &
		    \multicolumn{1}{c}{Hellenic} & 
			\multicolumn{1}{c}{Lexvo} & 
			\multicolumn{1}{c}{Tharawat}& 
			\multicolumn{1}{c}{Whisky} &
		    \multicolumn{1}{c}{World lift}\\\midrule
		    \multicolumn{2}{c|}{FKGE-simple} & 70.28 & 73.94 & 67.29 & 78.53 & 85.81 & 92.19 & 67.38 & 85.24 & 78.34 & 77.27 & 86.36\\
		    \multicolumn{2}{c|}{FKGE} & 71.22 & 75.34 & 67.69 & 79.27 & 86.41 & 93.70 & 68.24 & 85.71 & 78.75 & 79.55 & 89.09\\\midrule
		\end{tabular}
	}\caption{Evaluation results of FKGE on triple classification with two different aggregation setting (\%).}\label{tab:fkge-seting}
\vspace{-7mm}
\end{table*}

\section{Scale Experiments}
\label{Appendix-Scale}
%\subsubsection{Scale of Aligned Entities}
In order to measure the impact of the scale of aligned entities involved in the FKGE, we compare the performance of different numbers of the aligned entities and different numbers of knowledge graphs under triple classification.
We randomly sample 20\%, 40\%, 60\% and 80\% of the aligned entities for fusing them through the \ph{PPAT network}, respectively.
The results on triple classification with different sampling rates are shown in Fig.~\ref{fig:ablation}.
Intuitively, the more entities' embeddings that can be fused, the more obvious the improvements are.
For example, by sampling 20\%, 40\%, 60\% and 80\% and 100\% sampling rates, the \emph{World lift} gains 3.52\%, 4.05\%, 5.19\%, 6.44\% and 7.16\% improvements on the triple classification task, respectively.
Similarly, Fig.~\ref{fig:dimensions-fkge} presents performances of FKGE by setting 3 different dimensions of embedding vectors.
Overall, we can find that the larger the dimension of the embedding vector in the whole, the more obvious the effect that FKGE improves.
The reason may be that under a certain dimension ranges, the larger the dimension of the embedded vectors, the more hidden information FKGE can federate.

Tab.~\ref{tab:link-scale-filter} presents the results of link prediction by using TransE based FKGE, in terms of Mean Rank, Hit@10, Hit@3 and Hit@1, with different sampling ratio in the \ph{PPAT network}.
Intuitively, the more entities' embeddings that can be integrated, the more obvious the improvements are.
For example, 
in the Filter metric, by using the federated knowledge graph representation learning of 20\%, 40\%, 60\%, 80\% and 100\% (Presented in Tab.~\ref{tab:link-predict}) sampling rates, the \emph{Poképédia} gains up to 0.23\%, 5.11\%, 5.95\%, 7.35\% and 7.44\% improvements in terms of Hit@10 on the link prediction task, respectively.
In addition to the metric of Hit@10, most of other knowledge graphs have achieved similar performance improvements in Mean Rank, Hit@3 and Hit@1.
The above experimental results have once again proved the scalability and effectiveness of the proposed FKGE framework.

In order to measure whether the inclusion of virtual entities and relations contributes to the improvement of KGE, we compare the results of two types of aggregation methods on the triple classification task.
We name the FKGE without additional virtual entities and relations in the generated embedding of \ph{PPAT network} as FKGE-simple.
By using TransE as base KGE method, Tab. ~\ref{tab:fkge-seting} presents the result of triple classification between FKGE and FKGE-simple for all 11 knowledge graphs.
We observe the consistent increases from 0.40\% (Yago) to 2.73\% (World lift) by including virtual entities and relations in the FKGE.
%We observed that the virtual entities and relations added to FKGE help to achieve consistent increases from 0.42\% (Tharawat magazine) to 3.65\% (Sandrart) in current task.

%\subsubsection{Aggregation Functions}

%\section{Link prediction}
%\subsection{Evaluation results of Mean Rank}
